# Supplementary material for: FACTUAL: A Benchmark for Faithful and Consistent Textual Scene Graph Parsing
Source: arXiv:2305.17497 source file (2023-06-01)
Supplement: Supplementary file 1 [file 7_appendix.tex]

\section{Appendix}
\label{sec:appendix}
\subsection{FACTUAL Grammar Description}
\label{sec:scene}
\begin{table*}[t]
    % \vspace{-1mm}

  \resizebox{\textwidth}{!}{%
  \begin{tabular}{l}
    \toprule

attr,obj, vb, prep, qt\\
expr = Relation(qt? quantifier, obj subject, vb? verb, prep? preposition, qt? quantifier, obj object) \\
|Attribute(obj subject, attr attribute)\\
    | And(expr* arguments)\\
    \bottomrule
  \end{tabular}%
  }
    \caption{The grammar in ASDL for our scene graph annotations 
     \vspace{-3mm} }
  \label{tab:adsl}
    \vspace{-3mm}
\end{table*}
